# Supplementary material for: Curriculum Dataset Distillation
Source: arXiv:2405.09150 source file (2025-07-11)
Supplement: Supplementary file 1 [file supp.tex]

\documentclass[lettersize,journal]{IEEEtran}
\usepackage{amsmath,amsfonts}
\usepackage{algorithmic}
\usepackage{algorithm}
\usepackage{array}
\usepackage[caption=false,font=normalsize,labelfont=sf,textfont=sf]{subfig}
\usepackage{textcomp}
\usepackage{stfloats}
\usepackage{url}
\usepackage{verbatim}
\usepackage{graphicx}
\usepackage{cite}
\hyphenation{op-tical net-works semi-conduc-tor IEEE-Xplore}
% updated with editorial comments 8/9/2021

\usepackage{multirow}
\usepackage{graphicx}
\usepackage{amsmath}
\usepackage{amssymb}
\usepackage{mathtools, nccmath}
\usepackage{amsthm}
\usepackage{pifont}

\usepackage{algorithm, algorithmic}
\usepackage{graphicx}
\usepackage{wrapfig, lipsum, booktabs}
\usepackage{colortbl}
\usepackage{comment}
\usepackage{cleveref}
\usepackage{marvosym}
\usepackage{enumitem}
\usepackage{tabularx}
\usepackage{nicematrix}
\usepackage{caption}
\usepackage{diagbox}
\usepackage{dsfont}
\usepackage{natbib}

\begin{document}

\title{Curriculum Dataset Distillation}
\author{Zhiheng Ma\textsuperscript{*},
        Anjia Cao\textsuperscript{*},
        Funing Yang,
        Xing Wei\textsuperscript{\dag}
\IEEEcompsocitemizethanks{\IEEEcompsocthanksitem The authors are with Shenzhen University of Advanced Technology, China, School of Software Engineering, Xi'an Jiaotong University, China (Email: zh.ma@siat.ac.cn, \{caoanjia7, moolink\}@stu.xjtu.edu.cn, and weixing@mail.xjtu.edu.cn).
\IEEEcompsocthanksitem $*$: Equal Contribution.%
\IEEEcompsocthanksitem $\dag$: Corresponding Author.}% <-this % stops a space
}

\input{sections/appendix}

\vfill

\end{document}
